# Supplementary material for: Interactive Teaching Algorithms for Inverse Reinforcement Learning
Source: arXiv:1905.11867 source file (2019-06-05)
Supplement: Supplementary file 1 [file 8.0_appendix-table-of-contents.tex]

%!TEX root = main.tex
%%%%%%%%%%%%%%%%%%%%%%%%%%%%%%%%%%%%%%%%%%%%%%%%%%%%%%%%%
\section{List of Appendices}\label{sec.appendix.table}
In this section we provide a brief description of the content provided in the appendices of the paper.   
\begin{itemize}
\item Appendix~\ref{sec.appendix.maxent} provides a brief overview of batch MCE-IRL algorithm \cite{ziebart2010modeling}. 
\item Appendix~\ref{sec.appendix.policy-hyper-teaching} formally shows that teaching the policy $\pi^E$ to the learner is roughly equivalent to teaching a corresponding hyperparameter $\lambda^*$.   
\item Appendix~\ref{sec.appendix.maxent-assistive-teaching} provides proofs of teaching complexity results for the omniscient teaching setting.
\end{itemize}
