# Supplementary material for: Interactive Teaching Algorithms for Inverse Reinforcement Learning
Source: arXiv:1905.11867 source file (2019-06-05)
Supplement: Supplementary file 2 [file 8.4_appendix-temp.tex]

%!TEX root = main.tex
%%%%%%%%%%%%%%%%%%%%%%%%%%%%%%%%%%%%%%%%%%%%%%%%%%%%%%%%%

\section{TEMP --- Gradient Computation for Sequential MCE-IRL}\label{sec.appendix.maxent}
In this section, we compute the gradient $g_t$ for the sequential MCE-IRL learner at time $t$. As mentioned in Section~\ref{sec.omni-teaching}, we consider a learner update rule given by $\lambda_{t+1} ~=~ \lambda_t - \eta_t g_t$ with $g_t$ given by 
\[
g_t ~=~ \sum_{s,a} \bss{\rho^{\pi^L_t , s_{t,0}} \brr{s,a} - \rho^{\xi_t} \brr{s,a}} \nabla_\lambda R^L_\lambda \brr{s,a} \big \vert_{\lambda = \lambda_t} .
\]
The following proposition shows that $g_t$ is the gradient of the discounted negative log-likelihood of teacher's demonstration $\xi_t$. 

\begin{proposition}
\label{mce-gradient-proposition}
Given a demonstration $\xi = \bcc{\brr{s_{\tau}, a_{\tau}}}_{\tau=0,1,\dots}$, define
\begin{equation*}
c\brr{\lambda ; \xi} ~:=~ - \sum_\tau \gamma^\tau \log \pi^L_\lambda \brr{a_{\tau} \mid s_{\tau}} .
\end{equation*}
Then the gradient of $c\brr{\lambda ; \xi}$ w.r.t. $\lambda$ is given by 
\[
\nabla_\lambda c\brr{\lambda ; \xi} ~=~ \sum_{s,a} \bss{\rho^{\pi^L_\lambda} \brr{s,a} - \rho^{\xi} \brr{s,a}} \nabla_\lambda R^L_\lambda \brr{s,a} .
\]
\end{proposition}

$\mathbb{I}\bcc{s_\tau = s , a_\tau = a}$

\begin{proof}
First, we rewrite $c\brr{\lambda ; \xi}$ as follows:

\begin{align*}
c\brr{\lambda ; \xi} ~=~& - \sum_{\tau = 0}^{\infty} \sum_{s , a} \mathbb{I}\bcc{s_\tau = s , a_\tau = a} \gamma^\tau \bss{Q_\lambda \brr{s, a} - V_\lambda \brr{s}} \\
~=~& \textcolor{red}{V_\lambda \brr{s_0}}  \\
& \textcolor{blue}{- Q_\lambda \brr{s_0, a_0} + \gamma \sum_{s'} T(s' \mid s_0 , a_0) V_\lambda \brr{s'}} \\
& \textcolor{magenta}{- \gamma Q_\lambda \brr{s_1, a_1} + \gamma^2 V_\lambda \brr{s_2}} \\
& \textcolor{violet}{- \gamma^2 Q_\lambda \brr{s_2, a_2} + \gamma^3 V_\lambda \brr{s_3}} \\ 
& \dots .
\end{align*}


\begin{align*}
c\brr{\lambda ; \xi} ~=~& - \sum_{\tau = 0}^{\infty} \sum_{s , a} \mathbb{I}\bcc{s_\tau = s , a_\tau = a} \gamma^\tau \bss{Q_\lambda \brr{s, a} - V_\lambda \brr{s}} \\
~=~& \textcolor{red}{V_\lambda \brr{s_0}}  \\
& \textcolor{blue}{- Q_\lambda \brr{s_0, a_0} + \gamma V_\lambda \brr{s_1}} \\
& \textcolor{magenta}{- \gamma Q_\lambda \brr{s_1, a_1} + \gamma^2 V_\lambda \brr{s_2}} \\
& \textcolor{violet}{- \gamma^2 Q_\lambda \brr{s_2, a_2} + \gamma^3 V_\lambda \brr{s_3}} \\ 
& \dots .
\end{align*}
We will make use of the following quantities as part of the proof:
\begin{itemize}
    \item $P^L_{\tau}\brr{s}$ is defined as ...
    \item $P^L_{\tau}\brr{s, a}$ is defined as ...
\end{itemize}
To begin, we have $P^L_{0}\brr{s} = 1 \textnormal{ for } s = s_0$.
Now, we compute the gradient of the \textcolor{red}{first term}: 
\begin{align*}
\nabla_\lambda V_\lambda \brr{s_0} ~=~& \nabla_\lambda \sum_{s} P^L_{0}\brr{s} V_\lambda \brr{s} \\
~=~& \sum_{s} P^L_{0}\brr{s} \nabla_\lambda V_\lambda  \brr{s} \\
~=~& \sum_{s} P^L_{0}\brr{s} \nabla_\lambda \log \sum_{a}{\exp \brr{ Q_\lambda \brr{s, a} }} \\
~=~& \sum_{s} P^L_{0}\brr{s} \frac{\sum_{a}{\exp \brr{ Q_\lambda \brr{s, a} } \nabla_\lambda Q_\lambda \brr{s, a}}}{\sum_{a}{\exp \brr{ Q_\lambda \brr{s, a} }}} \\
~=~& \sum_{s} P^L_{0}\brr{s} \sum_{a} \pi^L_{\lambda} (a \mid s) \nabla_\lambda Q_\lambda \brr{s, a} \\
~=~& \sum_{s , a} P^L_0\brr{s , a} \bss{\nabla_\lambda R^L_\lambda \brr{s, a} + \gamma \sum_{s'}{T(s' \mid s , a) \nabla_\lambda V_\lambda \brr{s'}}} \\
~=~& \sum_{s , a} P^L_0\brr{s , a} \nabla_\lambda R^L_\lambda \brr{s, a} + \sum_{s'} \sum_{s , a} P^L_0\brr{s , a} T(s' \mid s , a) \gamma \nabla_\lambda V_\lambda \brr{s'} \\
~=~& \sum_{s , a} P^L_0\brr{s , a} \nabla_\lambda R^L_\lambda \brr{s, a} + \sum_{s'} P^L_1\brr{s'} \gamma \nabla_\lambda V_\lambda \brr{s'} \\
~=~& \sum_{s , a} P^L_0\brr{s , a} \nabla_\lambda R^L_\lambda \brr{s, a} + \sum_{s' , a'} P^L_1\brr{s' , a'} \gamma \nabla_\lambda R^L_\lambda \brr{s', a'} + \dots \\
~=~& \sum_{s , a} \sum_{\tau = 0}^{\infty} \gamma^\tau P^L_\tau \brr{s,a} \nabla_\lambda R^L_\lambda \brr{s , a} \\
~=~& \sum_{s , a} \rho^{\pi^L_\lambda , s_0} \brr{s,a} \nabla_\lambda R^L_\lambda \brr{s , a} . 
\end{align*}

We will make use of the following quantities as part of the proof:
\begin{itemize}
    \item $P^E_{\tau}\brr{s}$ is defined as $\mathbb{I}\bcc{s_\tau = s}$
    \item $P^E_{\tau}\brr{s, a}$ is defined as $\mathbb{I}\bcc{s_\tau = s , a_\tau = a}$
\end{itemize}

Now, we compute the gradient of the \textcolor{blue}{second term}: 
\begin{align*}
& - \nabla_\lambda Q_\lambda \brr{s_0, a_0} + \gamma \nabla_\lambda V_\lambda \brr{s_1} \\
~=~& - \sum_{s , a} P^E_0\brr{s , a} \nabla_\lambda Q_\lambda \brr{s, a} + \gamma \sum_{s'} P^E_1\brr{s'} \nabla_\lambda V_\lambda \brr{s'} \\
~=~& - \sum_{s , a} P^E_0\brr{s , a} \bss{\nabla_\lambda R^L_\lambda \brr{s, a} + \gamma \sum_{s'}{T(s' \mid s , a) \nabla_\lambda V_\lambda \brr{s'}}} + \gamma \sum_{s'} P^E_1\brr{s'} \nabla_\lambda V_\lambda \brr{s'} \\
~=~& - \sum_{s , a} P^E_0\brr{s , a} \nabla_\lambda R^L_\lambda \brr{s, a} - \gamma \sum_{s'} \sum_{s , a} P^E_0\brr{s , a} T(s' \mid s , a) \nabla_\lambda V_\lambda \brr{s'} + \gamma \sum_{s'} P^E_1\brr{s'} \nabla_\lambda V_\lambda \brr{s'} \\
%~=~& - \sum_{s_0 , a_0} P^E\brr{s_0 , a_0} \nabla_\lambda R^L_\lambda \brr{s_0, a_0} - \gamma \sum_{s_1} P^E\brr{s_1} \nabla_\lambda V_\lambda \brr{s_1} + \gamma \sum_{s_1} P^E\brr{s_1} \nabla_\lambda V_\lambda \brr{s_1} \\
%~=~& - \sum_{s_0 , a_0} P^E\brr{s_0 , a_0} \nabla_\lambda R^L_\lambda \brr{s_0, a_0} .
\end{align*}


\begin{align*}
& - \gamma \nabla_\lambda Q_\lambda \brr{s_1, a_1} + \gamma^2 \nabla_\lambda V_\lambda \brr{s_2} \\
~=~& - \gamma \sum_{s , a} P^E_1\brr{s , a} \nabla_\lambda Q_\lambda \brr{s, a} + \gamma^2 \sum_{s'} P^E_2\brr{s'} \nabla_\lambda V_\lambda \brr{s'} \\
~=~& - \gamma \sum_{s , a} P^E_1\brr{s , a} \bss{\nabla_\lambda R^L_\lambda \brr{s, a} + \gamma \sum_{s'}{T(s' \mid s , a) \nabla_\lambda V_\lambda \brr{s'}}} + \gamma^2 \sum_{s'} P^E_2\brr{s'} \nabla_\lambda V_\lambda \brr{s'} \\
~=~& - \gamma \sum_{s , a} P^E_1\brr{s , a} \nabla_\lambda R^L_\lambda \brr{s, a} - \gamma^2 \sum_{s'} \sum_{s , a} P^E_1\brr{s , a} T(s' \mid s , a) \nabla_\lambda V_\lambda \brr{s'} + \gamma^2 \sum_{s'} P^E_2\brr{s'} \nabla_\lambda V_\lambda \brr{s'} \\
%~=~& - \sum_{s_0 , a_0} P^E\brr{s_0 , a_0} \nabla_\lambda R^L_\lambda \brr{s_0, a_0} - \gamma \sum_{s_1} P^E\brr{s_1} \nabla_\lambda V_\lambda \brr{s_1} + \gamma \sum_{s_1} P^E\brr{s_1} \nabla_\lambda V_\lambda \brr{s_1} \\
%~=~& - \sum_{s_0 , a_0} P^E\brr{s_0 , a_0} \nabla_\lambda R^L_\lambda \brr{s_0, a_0} .
\end{align*}



By following similar steps, the gradient of all the terms except the \textcolor{red}{first term} is given by
\[
- \sum_{\tau = 0}^{\infty} \sum_{s_\tau , a_\tau} P^E\brr{s_\tau , a_\tau} \gamma^\tau \nabla_\lambda R^L_\lambda \brr{s_\tau, a_\tau} ~=~ - \sum_{s , a} \rho^{\xi} \brr{s,a} \nabla_\lambda R^L_\lambda \brr{s , a} . 
\]
Thus the full gradient is given by
\[
\nabla_\lambda c\brr{\lambda ; \xi} ~=~ \sum_{s,a} \bss{\rho^{\pi^L_\lambda} \brr{s,a} - \rho^{\xi} \brr{s,a}} \nabla_\lambda R^L_\lambda \brr{s,a} .
\]
\end{proof}


%In this section, we present the batch MCE-IRL algorithm, and prove the Proposition~\ref{mce-prop} and Proposition~\ref{mce-prop-linear}.

%\subsection{Background}
%Consider the MDP $\mathcal{M}$ with \emph{stochastic} state transition dynamics. The following is the reduction of the general maximum causal entropy optimization problem for this special case \cite{bloem2014infinite}:
%\begin{equation}
%\begin{aligned}
%& \underset{\pi^L (a \mid s)}{\text{minimize}}
%& & H(A_{0:\infty} || S_{0:\infty}) = \sum_{t=0}^\infty{\gamma^{t} H(A_t \mid A_{1:t-1}, S_{1:t})} \\
%& \text{subject to}
%& & \rho^{\pi^{L}} \brr{s,a} = \rho^{\Xi} \brr{s,a} , \quad \forall{s,a \in \mathcal{S} \times \mathcal{A}} \\
%&&& \sum_{a}{\pi^L (a \mid s)} = 1, \quad \pi^L (a \mid s) > 0 ,
%\end{aligned}
%\label{max-causal-ent-optimization}
%\end{equation}

%The solution to the above problem can be given in a parametric form \cite[Corollary~6.5]{ziebart2010modeling} as follows: 
%\begin{align*}
%\pi_{\lambda} (A_t \mid S_t) ~=~& \exp \brr{Q_\lambda \brr{S_t, A_t} - V_\lambda \brr{S_t}} \\
%V_\lambda \brr{S_t}  ~=~& \log \sum_{A_t}{\exp \brr{ Q_\lambda \brr{S_t, A_t} }} \\
%~=~& \mathrm{softmax}_{A_t} \brr{R^L_\lambda \brr{S_t, A_t} + \gamma \sum_{S_{t+1}}{T(S_{t+1} \mid S_t , A_t) V_\lambda \brr{S_{t+1}}}} \\
%~=~& \mathrm{softmax}_{A_t} \brr{R^L_\lambda \brr{S_t, A_t} + \gamma \mathbb{E}_{T(S_{t+1} \mid S_t , A_t)}\bss{V_\lambda \brr{S_{t+1}}}} \\
%Q_\lambda \brr{S_t, A_t} ~=~& R^L_\lambda \brr{S_t, A_t} + \gamma \sum_{S_{t+1}}{T(S_{t+1} \mid S_t , A_t) V_\lambda \brr{S_{t+1}}} \\
%~=~& R^L_\lambda \brr{S_t, A_t} + \gamma \mathbb{E}_{T(S_{t+1} \mid S_t , A_t)}\bss{V_\lambda \brr{S_{t+1}}} ,
%\end{align*}
%where $\mathrm{softmax}_{x} f(x) := \log \sum_x \exp(f(x))$, and the optimal parameter $\lambda_{\Xi}$ \cite[Theorem~6.4]{ziebart2010modeling} is given by: 
%\begin{align*}
%\lambda_{\Xi} ~=~& \argmax_{\lambda} \Pi_{i=1}^m \Pi_{t=0}^\infty \pi_{\lambda} (A_t^i \mid S_t^i) \\ 
%~=~& \argmax_{\lambda} \sum_{i,t} \log{\pi_{\lambda} (A_t^i \mid S_t^i)} =: c\brr{\lambda ; \Xi}
%\end{align*}

%\subsubsection{Gradient descent}  
%Consider that the learner's current parameter is $\lambda_\graditer$, and $\pi^{\lambda_\graditer}$ is the optimal policy for $\mathcal{M} \backslash R$ with $R_{\lambda_\graditer}\brr{s,a}$ computed via Soft-Value-Iteration procedure, \emph{cf.} \cite[Algorithm.~9.1]{ziebart2010modeling}. Then, the gradient of the above optimization problem is $g_\graditer = \frac{\partial c}{\partial \lambda} \big \vert_{\lambda = \lambda_\graditer} = \frac{\partial c}{\partial R^L_\lambda} \cdot \frac{\partial R^L_\lambda}{\partial \lambda} \big \vert_{\lambda = \lambda_\graditer} = \sum_{s,a} \bcc{\rho^{\Xi} \brr{s,a} - \rho^{\pi^{\lambda_\graditer}} \brr{s,a}} \frac{\partial R^L_\lambda \brr{s,a}}{\partial \lambda} \big \vert_{\lambda = \lambda_\graditer} \in \partial c\brr{\lambda_\graditer ; \Xi}$ \cite[Eq.~10.1]{ziebart2010modeling}. Thus the gradient descent update rule is given by:
%\[
%\lambda_{\graditer+1} \leftarrow \lambda_\graditer - \eta_\graditer \sum_{s,a} \bcc{\rho^{\pi_\graditer} \brr{s,a} - \rho^{\Xi} \brr{s,a}} \frac{\partial R^L_\lambda \brr{s,a}}{\partial \lambda} \bigg \vert_{\lambda = \lambda_\graditer} ,
%\]
%where $\pi_\graditer ~:= \pi^{\lambda_\graditer}$ and $\eta_\graditer$ denotes the current learning rate. 

%\subsection{Batch MCE-IRL}
%where $\pi_t$ is the optimal policy w.r.t. $\lambda_t$. 
%
%
%xxx where $\pi_t = \pi^{\lambda_t}$ is the optimal policy for $\mathcal{M} \backslash R$ with $R(s) = \ipp{\lambda_t}{\phi(s)}$ computed via Soft-Value-Iteration procedure, cf. \cite[Algorithm.~9.1]{ziebart2010modeling}. The following proposition shows that teaching the optimal solution of the problem~\eqref{batch-mce-opt} to the learner, with an appropriate set of demonstrations, is sufficient to achieve the learner's objective. xxx

%The MCE-IRL approach can be interpreted (in dual form) as maximizing the causal likelihood of the demonstration data. 

%%%%%%%%%%%%%%%%%%%%%%%%%%%%%%%%%%%%%%%%%%%%%%%%%%%%%%%%%%%%%%%
%%%%%%%%%%%%%%%%%%%%%%%%%%%%%%%%%%%%%%%%%%%%%%%%%%%%%%%%%%%%%%%
%%%%%%%%%%%%%%%%%%%%%%%%%%%%%%%%%%%%%%%%%%%%%%%%%%%%%%%%%%%%%%%
%%%%%%%%%%%%%%%%%%%%%%%%%%%%%%%%%%%%%%%%%%%%%%%%%%%%%%%%%%%%%%%
%%%%%%%%%%%%%%%%%%%%%%%%%%%%%%%%%%%%%%%%%%%%%%%%%%%%%%%%%%%%%%%
%%%%%%%%%%%%%%%%%%%%%%%%%%%%%%%%%%%%%%%%%%%%%%%%%%%%%%%%%%%%%%% Background
% \subsection{Learner Model with Generic Reward Function} \label{sec:learner.model.generic}
% For two matrices $A$ and $B$, we define $\ipp{A}{B} := \sum_{i}\sum_{j} A_{i,j} B_{i,j}$. Given a finite MDP $\mathcal{M}$ with $\mathcal{S} = \bcc{1,2,\ldots,\abs{\mathcal{S}}}$, and $\mathcal{A} = \bcc{1,2,\ldots,\abs{\mathcal{A}}}$, we consider a learner model with generic reward function $R^L_\lambda (s,a) = \ipp{\lambda}{\phi^L(s,a)}$ where $\lambda$ is a $\abs{\mathcal{S}} \times \abs{\mathcal{A}}$ matrix and $\phi^L(s,a)$ is given by
% \[
% \bss{\phi^L(s,a)}_{i,j} ~:=~ \begin{cases}
%                         1 \quad \text{when $i=s$, and $j=a$} \\
%                         0 \quad \text{otherwise}
%                     \end{cases} 
% \]
% Given a collection of demonstrations $\Xi = \bcc{\xi_t}_{t=1,2,\dots}$ (where $\xi_t = \bcc{\brr{s_{t,\tau}, a_{t,\tau}}}_{\tau=0,1,\dots}$), the batch MCE-IRL algorithm (with the above learner model) is formulated by the following dual optimization problem \cite[Theorem~6.4]{ziebart2010modeling}:
% \begin{equation}
% \underset{\lambda}{\mathrm{maximize}} ~~ c\brr{\lambda ; \Xi} ~:=~ \sum_t \sum_\tau \log \pi^L_\lambda \brr{a_{t,\tau} \mid s_{t,\tau}} ,
% \label{c-func-generic}
% \end{equation}
% where the parametric policy $\pi^L_{\lambda}$ \cite[Corollary~6.5]{ziebart2010modeling} is given by
% \begin{align*}
% \pi^L_{\lambda} (a \mid s) ~=~& \exp \brr{Q_\lambda \brr{s, a} - V_\lambda \brr{s}} \\
% V_\lambda \brr{s}  ~=~&\log \sum_{a}{\exp \brr{ Q_\lambda \brr{s, a} }} \\
% Q_\lambda \brr{s, a} ~=~& R^L_\lambda \brr{s, a} + \gamma \sum_{s'}{T(s' \mid s , a) V_\lambda \brr{s'}}.  
% \end{align*}
% The resulting batch MCE-IRL algorithm is given in Algorithm~\ref{algo:batch-max-ent-irl}, which is an instantiation of Algorithm~\ref{algo:batch-max-ent-irl-common}.

% \paragraph{Primal Problem.} The corresponding primal problem (with occupancy measure matching) for the above dual problem Eq.~\eqref{c-func-generic} is given by \cite{bloem2014infinite}:
% \begin{equation}
% \begin{aligned}
% & \underset{\pi^L (a \mid s)}{\text{maximize}}
% & & \sum_{\tau=0}^\infty{\gamma^{\tau} H(a_\tau \mid a_{0:\tau-1}, s_{0:\tau})} \\
% & \text{subject to}
% & & \rho^{\pi^L} \brr{s,a} = \rho^{\Xi} \brr{s,a} , \,\, \forall{s,a \in \mathcal{S} \times \mathcal{A}} \\
% &&& \sum_{a}{\pi^L (a \mid s)} = 1, \, \, \pi^L(a \mid s) \geq 0 ,
% \end{aligned}
% \label{max-causal-ent-optimization}
% \end{equation}
% where $H$ is the conditional entropy. 

% \begin{algorithm}
%     \caption{Batch MCE-IRL (Generic Reward)}\label{algo:batch-max-ent-irl}
% 	\begin{algorithmic}
% 	    \State \textbf{Input:} collection of demonstrations $\Xi$ \;
%         \State \textbf{Initialization:} $\lambda_1$ and $\pi^L_1$ \;
%         \For{$\graditer=1,2,\dots$}
%             \State $\lambda_{\graditer+1} \gets \lambda_{\graditer} - \eta_\graditer \sum_{s,a} \bcc{\rho^{\pi^L_\graditer} \brr{s,a} - \rho^{\Xi} \brr{s,a}} \phi^L(s,a)$ \;
%             \State $\pi^L_{\graditer+1} \gets \textnormal{Soft-Value-Iteration}\brr{\mathcal{M} \textbackslash R^E, R^L_{\lambda_{\graditer+1}}}$ \;
%         \EndFor
%   %\KwResult{policy $\pi^L \gets \pi_T$}
% 	\end{algorithmic}
% \end{algorithm}

% \subsection{Learner Model with Linear Reward Function}
% \label{sec:learner.model.linear}
% Here, we consider a learner model with linear reward function $R^L_\lambda (s,a) = \ipp{\lambda}{\phi^L(s,a)}$ where $\lambda \in \mathbb{R}^d$ and $\phi^L(s,a) \in \mathbb{R}^d \, \forall{s,a}$. Given a collection of demonstrations $\Xi = \bcc{\xi_t}_{t=1,2,\dots}$ (where $\xi_t = \bcc{\brr{s_{t,\tau}, a_{t,\tau}}}_{\tau=0,1,\dots}$), the batch MCE-IRL algorithm (with the above learner model) is formulated by the following dual optimization problem \cite[Theorem~6.4]{ziebart2010modeling}:
% \begin{equation}
% \underset{\lambda}{\mathrm{maximize}} ~~ c\brr{\lambda ; \Xi} ~:=~ \sum_t \sum_\tau \log \pi^L_\lambda \brr{a_{t,\tau} \mid s_{t,\tau}} ,
% \label{c-func-linear}
% \end{equation}
% where the parametric policy $\pi^L_{\lambda}$ \cite[Corollary~6.5]{ziebart2010modeling} is given by
% \begin{align*}
% \pi^L_{\lambda} (a \mid s) ~=~& \exp \brr{Q_\lambda \brr{s, a} - V_\lambda \brr{s}} \\
% V_\lambda \brr{s}  ~=~&\log \sum_{a}{\exp \brr{ Q_\lambda \brr{s, a} }} \\
% Q_\lambda \brr{s, a} ~=~& R^L_\lambda \brr{s, a} + \gamma \sum_{s'}{T(s' \mid s , a) V_\lambda \brr{s'}}.  
% \end{align*}
% The resulting batch MCE-IRL algorithm (with $\mu^{\pi^L} = \sum_{s,a} \rho^{\pi^L} (s,a) \phi^L (s,a)$, and $\mu^{\Xi} = \sum_{s,a} \rho^{\Xi} (s,a) \phi^L (s,a)$) is given in Algorithm~\ref{algo:batch-max-ent-irl-linear}, which is an instantiation of Algorithm~\ref{algo:batch-max-ent-irl-common}.

% \paragraph{Primal Problem.} The corresponding primal problem (with feature expectation matching) for the above dual problem Eq.~\eqref{c-func-linear} is given by \cite{bloem2014infinite}:
% \begin{equation}
% \begin{aligned}
% & \underset{\pi^L (a \mid s)}{\text{maximize}}
% & & \sum_{\tau=0}^\infty{\gamma^{\tau} H(a_\tau \mid a_{0:\tau-1}, s_{0:\tau})} \\
% & \text{subject to}
% & & \mu^{\pi^L} = \mu^{\Xi} \\
% &&& \sum_{a}{\pi^L (a \mid s)} = 1, \, \, \pi^L(a \mid s) \geq 0 ,
% \end{aligned}
% \label{max-causal-ent-optimization-linear}
% \end{equation}
% where $H$ is the conditional entropy. 


% \begin{algorithm}
%     \caption{Batch MCE-IRL (Linear Reward)}\label{algo:batch-max-ent-irl-linear}
% 	\begin{algorithmic}
% 	    \State \textbf{Input:} collection of demonstrations $\Xi$ \;
%         \State \textbf{Initialization:} $\lambda_1$ and $\pi^L_1$ \;
%         \For{$\graditer=1,2,\dots$}
%             \State $\lambda_{\graditer+1} \gets \lambda_{\graditer} - \eta_\graditer \sum_{s,a} \brr{\mu^{\pi^L_\graditer} - \mu^{\Xi}}$ \;
%             \State $\pi^L_{\graditer+1} \gets \textnormal{Soft-Value-Iteration}\brr{\mathcal{M} \textbackslash R^E, R^L_{\lambda_{\graditer+1}}}$ \;
%         \EndFor
%   %\KwResult{policy $\pi^L \gets \pi_T$}
% 	\end{algorithmic}
% \end{algorithm}

% \subsection{Learner Model with Deep Neural Network (DNN) Reward Function}
% \label{sec:learner.model.dnn}

% Here, we consider a feature map $\Phi$ which takes $\phi^L(\cdot,\cdot) \in \mathbb{R}^{d'}$ as input, and is parameterized by the weights $W \in \mathbb{R}^{d_1}$ of a deep neural network, i.e., $\Phi\brr{\phi^L (\cdot,\cdot) ; W} \in \mathbb{R}^{d_2}$. Given $\alpha \in \mathbb{R}^{d_2}$, denote $\lambda = \brr{\alpha , W} \in \mathbb{R}^{d}$ with $d = d_1 + d_2$. Then for the learner model with reward function $R^L_{\lambda} (s,a) = \ipp{\alpha}{\Phi\brr{\phi^L (s,a) ; W}}$, we attempt to learn $\alpha$, and $W$ jointly. Given a collection of demonstrations $\Xi = \bcc{\xi_t}_{t=1,2,\dots}$ (where $\xi_t = \bcc{\brr{s_{t,\tau}, a_{t,\tau}}}_{\tau=0,1,\dots}$), the batch MCE-IRL algorithm (with the above learner model) is formulated by the following dual optimization problem \cite{wulfmeier2015maximum}:
% \begin{equation}
% \underset{\lambda}{\mathrm{maximize}} ~~ c\brr{\lambda ; \Xi} ~:=~ \sum_t \sum_\tau \log \pi^L_\lambda \brr{a_{t,\tau} \mid s_{t,\tau}} ,
% \label{c-func-deep}
% \end{equation}
% where the parametric policy $\pi^L_{\lambda}$ \cite[Corollary~6.5]{ziebart2010modeling} is given by
% \begin{align*}
% \pi^L_{\lambda} (a \mid s) ~=~& \exp \brr{Q_\lambda \brr{s, a} - V_\lambda \brr{s}} \\
% V_\lambda \brr{s}  ~=~&\log \sum_{a}{\exp \brr{ Q_\lambda \brr{s, a} }} \\
% Q_\lambda \brr{s, a} ~=~& R^L_\lambda \brr{s, a} + \gamma \sum_{s'}{T(s' \mid s , a) V_\lambda \brr{s'}}.  
% \end{align*}
% The resulting batch MCE-IRL algorithm (with $\mu_W^{\pi^L} := \sum_{s,a} \rho^{\pi^L} (s,a) \Phi\brr{\phi^L (s,a) ; W}$, and $\mu^{\Xi} := \sum_{s,a} \rho^{\Xi} (s,a) \Phi\brr{\phi^L (s,a) ; W}$) is given in Algorithm~\ref{algo:batch-max-ent-irl-deep}, which is an instantiation of Algorithm~\ref{algo:batch-max-ent-irl-common}.

% \paragraph{Primal Problem.} The corresponding primal problem for the above dual problem Eq.~\eqref{c-func-deep} is given by:
% \begin{equation}
% \begin{aligned}
% & \underset{\pi^L (a \mid s), W}{\text{maximize}}
% & & \sum_{\tau=0}^\infty{\gamma^{\tau} H(a_\tau \mid a_{0:\tau-1}, s_{0:\tau})} \\
% & \text{subject to}
% & & \mu_W^{\pi^L} = \mu_W^{\Xi} \\
% &&& \sum_{a}{\pi^L (a \mid s)} = 1, \, \, \pi^L(a \mid s) \geq 0 ,
% \end{aligned}
% \label{max-causal-ent-optimization-deep}
% \end{equation}
% where $H$ is the conditional entropy. 

% \begin{algorithm}
%     \caption{Batch MCE-IRL (DNN Reward)}\label{algo:batch-max-ent-irl-deep}
% 	\begin{algorithmic}
% 	    \State \textbf{Input:} collection of demonstrations $\Xi$ \;
%         \State \textbf{Initialization:} $\lambda_1$ and $\pi^L_1$ \;
%         \For{$\graditer=1,2,\dots$}
%             \State $\alpha_{\graditer+1} \gets \alpha_{\graditer} - \eta_\graditer \sum_{s,a} \bcc{\rho^{\pi^L_\graditer} \brr{s,a} - \rho^{\Xi} \brr{s,a}} \Phi\brr{\phi^L (s,a) ; W_\graditer}$ \;
%             \State $W_{\graditer+1} \gets W_{\graditer} - \eta_\graditer \sum_{s,a} \bcc{\rho^{\pi^L_\graditer} \brr{s,a} - \rho^{\Xi} \brr{s,a}} \frac{\partial R^L_{\lambda} \brr{s,a}}{\partial W} \big \vert_{\alpha = \alpha_\graditer , W = W_\graditer}$ \;
%             \State $\pi^L_{\graditer+1} \gets \textnormal{Soft-Value-Iteration}\brr{\mathcal{M} \textbackslash R^E, R^L_{\lambda_{\graditer+1}}}$ \;
%         \EndFor
%   %\KwResult{policy $\pi^L \gets \pi_T$}
% 	\end{algorithmic}
% \end{algorithm}
